# Supplementary material for: Explore User Neighborhood for Real-time E-commerce Recommendation
Source: arXiv:2103.00442 source file (2021-02-28)
Supplement: Supplementary file 1 [file appendix.tex]

\clearpage
\appendix

\section{INFORMATION FOR REPRODUCIBILITY}
\subsection{The preprocessing steps for datasets.}
For dataset preprocessing, we follow the common practice in~ \cite{he2017translation,kang2018self,Sedhain:2016:PLM:3061053.3061158}.
We convert all numeric ratings or presence of a review to ``1'' and others to ``0''. 
It is worth mentioning that for amazon datasets, we follow the preprocessing procedure from \citeauthor{he2017translation}~ \cite{he2017translation}, which discard users and items with fewer than 5 related actions. 
And then to guarantee each user with enough interactions, we discard users with fewer than 5 actions once more. 
The processed data statistics are summarized in Table~\ref{tab:dataset}.

\begin{table}
  \caption{Dataset statistics (after preprocessing)}
  \label{tab:dataset}
  \begin{tabular}{cccccc}
    \toprule
    Dataset &\#users &\#items &\#actions &avg.length & density\\
    \midrule
    ML-1M & 6040& 3416 &1.0M & 163.5 & 4.79\%\\
    ML-20M & 138493& 26744 &20M & 144.4 & 0.54\%\\
    Games & 29341& 23464&0.3M & 9.1 & 0.04\%\\
    Beauty & 40226 & 54542&0.4M & 8.8 & 0.02\%\\
  \bottomrule
\end{tabular}
\end{table}

\subsection{Implementation Details}
We implement BPR-MF, FISM, SASRec, and our SCCF with \texttt{TensorFlow}. 
When tuning the UI models, we hold out the item just before the last for each user as the validation set. 
To generate mini-batch for training FISM, we follow~\cite{he2018nais} that forms a mini-batch as all training instances of a randomly sampled user, rather than randomly sampling a fixed number of training instances as a mini-batch.
Meanwhile, we train FISM without regularization. 
If overfitting is observed, we then cope with it with early stop strategy.
However, when training SASRec model, we follows \citeauthor{kang2018self}~\cite{kang2018self} settings, which uses dropout mechanism to avoid overfitting.

To train the integrating model, we utilize each user's the item just before the last as the training label.
Then, we randomly split ten percent of the whole users as the validation set to tune the integrating model.
We apply the early stop strategy to avoid overfitting.
When measuring the performance on the test set, we add all validation items and users back to the training set, and derive the final model parameters.

\subsection{Parameter Settings}
All parameters are initialized by truncated normal distribution in the range $[-0.01, 0.01]$.
We optimize the model using the Adam optimizer with the learning rate of $0.001$, $\beta_1 = 0.9$, $\beta_2 = 0.999$, and linear decay of the learning rate.
For the embedding size $k$, we test the values of $[16, 32, 64, 128]$.
Meanwhile, we test the effect of the number of user neighbors of $[ 50, 100, 200]$.
We set $\alpha=0.5$ when training the FISM model and 
the SASRec parameter settings are the same as \citeauthor{kang2018self}~\cite{kang2018self} with the layer number of 2 and head number of 1.
For fair comparison, we use the same maximum sequence length as in~\cite{kang2018self}, for ML-1M and ML-20M $N=200$, and for Games and Beauty $N=50$.
Since users' interests are dynamically changed, for FISM method, we leverage the recent 15 items to infer user embedding.
And then for both methods, we recommend each user's latest 15 items to his/her similar user for user-based component. 

\section{Evidence for Online Experiments}
\subsection{Importance for Real-time Recommendation}
\begin{figure}
  \centering
  \includegraphics[width=0.9\linewidth]{barplot2.pdf}
  \caption{The average proportion of fine categories that users first clicked at each day. We collect the number of fine categories that each user clicks at one day. And each bar denotes the proportion of these categories users first clicked before this day.}
  \label{Realtime}
\end{figure}
We analyze the changes of users' interest by recording the proportion of fine categories that users have never clicked in two weeks before this day.
We collect the number of fine categories that each user clicks at one specific day. 
And then we look for the day users first clicked before this day.
The results are visualizing in Figure~\ref{Realtime}.
We observe that most of the categories that users click today are new categories that they do not click before today.
Therefore, we need to adapt to users' dynamic interest in real time to make better recommendations.
